# Supplementary material for: Prometheus 2: An Open Source Language Model Specialized in Evaluating Other Language Models
Source: arXiv:2405.01535 source file (2024-12-04)
Supplement: Supplementary file 1 [file appendix.tex]

/section(
